# Supplementary material for: CrisisLTLSum: A Benchmark for Local Crisis Event Timeline Extraction and Summarization
Source: arXiv:2210.14190 source file (2022-10-25)
Supplement: Supplementary file 2 [file additional.tex]

% Timeline summarization has also been investigated in other domains such as news~\cite{nallapati2016abstractive,narayan2018don,gusev2020dataset}, Reddit~\cite{kim2018abstractive}, academic papers~\cite{lo2019s2orc}, dialogues~\cite{gliwa2019samsum}, and tutorials~\cite{koupaee2018wikihow}. Again, except some~\cite{kim2018abstractive}, most of these domains have only focused on extractive summarization.
% Additionally, summarizing timelines extracted from Twitter is more challenging due to the amount of noise~\cite{alam2021humaid}, the poor language~\cite{rudra2018extracting}, and the high overlap of information described in multiple tweets~\cite{rudra2018extracting}.
% Compared to centralized sources such as news~\cite{nallapati2016abstractive}, tweets can provide more frequent and real-time updates while covering various angles of an ongoing event.


% As the main focus of our dataset is to enable future research on real-time timeline extraction for local crisis events, 

% The importance of crisis domain information gathering and its role in understanding them
% The rise in technology has provided tools such as Twitter, which provide new sources of real-time information~\cite{hua2012information}. Such real-time information can be used to detect and track global/local events~\cite{zhang2019tracking,mamo2021fine}. This available large data source can also be used for extracting historical information for studying known events~\cite{repp2018extracting}.
% The availability of information through Twitter in the early hours of an event compared to the traditional sources is of great importance for applications in news~\cite{repp2018extracting} and crisis~\cite{martinez2018twitter} domains.
% One of the domains which can widely benefit from both real-time information and historical data is the crisis domain~\cite{}. 
% Extracting real-time crisis-related events from microblogs such as Twitter is important as it provides time-sensitive information which enables first responders to understand an ongoing situation and plan relief efforts accordingly~\cite{sarter1991situation}.
% Furthermore, extracting related information to an event can lead to benefits such as preventing future disastrous events in high-threat areas, helping first responders better understand and evaluate each event, and enabling a more profound understanding of factors and consequences of crisis events. 
% Furthermore, real-time crisis monitoring through social media can help people track an ongoing event to either provide life-saving emergency alerts, avoid getting close to the threat areas, or analyze the risks on important assets affected by the disaster.
% Tweets may contain information about the location of an event, type of the event, the severity of the situation, time of the incident, its progress, overall report, and consequences. 
% Compared to centralized sources such as news~\cite{nallapati2016abstractive}, tweets can provide more frequent and real-time updates while covering various angles of an ongoing event. However, extracting such information from Twitter is more challenging due to the amount of noise~\cite{alam2021humaid} and the poor language~\cite{rudra2018extracting}.

% Here, we provide a new dataset on concrete crisis event timelines on local events.
% Recent research has vastly investigated extracting crisis event from Twitter~\cite{alam2018crisismmd,olteanu2014crisislex,alam2021crisisbench,imran2016twitter}.
% This new dataset resolves some of the shortcomings of the existing resources and further expands the applications of such information by proposing two new tasks of timeline correction and timeline summarization.
% First, most of the prior research focuses on the extraction task as historic data~\cite{} where relevant tweets to an already known event are extracted. Here, we extract such information by relaxing this assumption by assuming no access to known events. This will help close the gap between the data generation approach and the real-life applications of such systems. Obviously, detecting and following unknown disaster events in an online system is harder due to not having access to a set of known names or keywords related to the events.

% First, existing datasets~\cite{alam2018crisismmd,alam2021crisisbench,alam2021humaid,olteanu2014crisislex,imran2016twitter} mostly focus on extracting information about known large disaster events such as long-lasting hurricanes, large earthquakes, or wildfire.
% This has imposes two major limitations. First, there is a need to have a set of curated keyword for each event individually. Second, this can only enable further understanding on very big events while crisis domain also includes a lot of smaller sized and local events. To address the first challenge, we do not start by a set of known events and instead rely on more general usage keyword lists which enables real-time detection.
% Obviously, detecting and following unknown disaster events in an online system is harder due to not having access to a set of known names or keywords, related to the events.
% To remove the second limitation, we further extend the extraction pipeline to support local events such as "a fire in a building", traffic accidents, or local wildfires by relying on location augmentation techniques. This essentially imposes a harder extraction challenge as local information appear less frequent in the tweet stream, which makes it harder for conventional clustering methods to detect them as spikes or clusters.

% Second, the extracted data in current datasets are often noisy, contain redundancy, and have overloaded information~\cite{alam2021humaid}. To address this issue, prior research~\cite{alam2021humaid} has considered fine-grained classification annotation for categorizing the tweets into groups such as prayers, urgent needs, or missing people. Although, this is a good step toward filtering out some of the noisy data, the redundancy challenge still remains open. detecting redundancy in a set of tweets is especially harder than a simple pair-based search as the information of one tweet is usually covered not by only one individual tweet but by an aggregation of multiple ones.

% The noise and duplicate removal are crucial steps on real-time tracking of events where new information should not be missed as hundreds of relevant tweets are frequently being added to the story. Here, we employ two post-processing steps to remove noise and redundancy as much as possible and later conduct an annotation task aiming to clean the clusters further. 
% The results of the annotation task can be later used on real-time extraction systems to filter out unrelated or repetitive information.

% Lastly, this is the first twitter dataset that proposes the task of abstractive summaries for crisis events and provides multiple gold annotations. Summarizing tweets are generally harder than other sources of information, given poor-language, and the the high overlap of information described in multiple tweets~\cite{rudra2018extracting}.

% Our dataset will pave the way toward extracting information about a wider range of crisis events while increasing the quality of the extractions to produce a clean and concrete timeline from microblogs in real-time while avoiding repetitive information.

% In our proposed dataset, each crisis event is called a timeline as it is represented by a chronologically sorted sequence of tweets. In contrast to the existing crisis datasets where each cluster contains every related tweet to the event, each tweet in our timelines should bring a new and important update to the story. This results in a clean timeline where the event and its progress is described clearly and is tractable. This can enable future research toward creating online systems for detecting crisis events and tracking them for updates as the event is progressing.

% We employ a two step strategy to create this dataset. First, we design an online clustering pipeline which extracts and clusters the tweet stream into a set of generated timelines. Second, we design an annotation task where a combination of experts and workers are asked to clean the generated timelines through a set of carefully designed tasks. We discuss the first step in Section \ref{sec:generate} and the annotation platform in Section \ref{sec:correct}. 
% Given the designed annotation task, we provide the following information about each tweet in the timeline. First, we specify whether each tweet belongs to the timeline. A tweet only belongs to the timeline, if it is related to the ongoing local story and provides a new information which has not been seen in any of the prior tweets. Second, if a tweet does not belong to the timeline, we provide a reason for the exclusion among not being related, not being informative, or not containing any new information.
% We further propose two tasks of timeline correction and timeline summarization in this dataset. The former task is to detect whether a tweet belongs to a given timeline and the reason of exclusion in case the tweet does not. The latter task is to generate a summary given a clean timeline of an event. 
